# Supplementary material for: Signaling in Posted Price Auctions
Source: arXiv:2201.12183 source file (2022-03-29)
Supplement: Supplementary file 1 [file appendix.tex]

\section{Appendix}

\subsection{Payment Function}
In the main paper, we consider a deterministic and factorized payment function $f:\mathcal{S}\rightarrow[0,1]^n$ such that $f(\svec)=(f^i(s_i))_{i \in \rec}$. Now we prove in two steps that this assumption is general. First, we show that for every stochastic payment function $g$ and signaling scheme $\mathcal{S}^g \coloneqq \bigtimes_{i \in \mathcal{N}} \mathcal{S}^g_i$ we can find a factorized stochastic payment function $h$ and a signaling scheme $\mathcal{S}^h \coloneqq \bigtimes_{i \in \mathcal{N}} \mathcal{S}^h_i$ which induce the same posted price auction. This means that the two scenarios provide the same revenue to the seller and the same posterior believes to the buyers. Then, we show that, given a signaling scheme $\mathcal{S}^h$ and a factorized stochastic payment function $h$, we can always find another signaling scheme $\mathcal{S}$ and a factorized deterministic payment function $f$ inducing the same posted price auction.

\paragraph{Notation}
\begin{itemize}
\item $\mathcal{P}=[0,1]^n$ set of price vectors $\boldsymbol{p} \in [0,1]^n$
\item $g:\mathcal{S}\rightarrow[0,1]^n$ stochastic payment function
\item $\pi^g:\mathcal{S}\rightarrow \Delta^{|\mathcal{P}|}$ probability distribution induced by function $g$ over the prices vectors  
\item $\pi^g_{s}[\boldsymbol{p}]$ probability of price vector $\boldsymbol{p}$ when the signal profile is $s \in \mathcal{S}$ and the payment function is $g$
\item $h:\mathcal{S}\rightarrow[0,1]^n$ s.t. $h(\svec)=(h^i(s_i))_{i \in \rec}$ factorized stochastic payment function 
\item $\pi^h:(\mathcal{S}_i)_{i\in\mathcal{R}}\rightarrow \Delta^{|\mathcal{P}|}$ probability distribution induced by function $h$ over the prices vectors
\item $\pi^{h_i}:\mathcal{S}_i\rightarrow \Delta$ probability distribution induced by function $h_i$ over the prices $\boldsymbol{p}[i]$ 
\item $\pi^{h}_{s_i}[p_i]$ probability of price $\boldsymbol{p}[i]=p_i$ when the signal is $s_i \in \mathcal{S}_i$ and the payment function is $h_i$ for buyer $i$
\item $f:\mathcal{S}\rightarrow[0,1]^n$ s.t. $f(\svec)=(f^i(s_i))_{i \in \rec}$ factorized deterministic payment function
\item $\boldsymbol{\xi}^g_{i, (s_i,p_i)} \in \Delta^{|\Theta|}$ posterior belief of a buyer $i \in \mathcal{N}$ upon receiving signal $s_i \in \mathcal{S}_i$ and price $\boldsymbol{p}[i]=p_i \in [0,1]$ when the price function is $g$, formally
\[
\boldsymbol{\xi}^g_{i, (s_i',p_i')}[\theta]=\frac{\boldsymbol{\mu}[\theta] \sum_{\boldsymbol{p} \in \mathcal{P} : \boldsymbol{p}[i] = p_i'} \sum_{s^g \in \mathcal{S}^g : s^g_i = s_i'} \boldsymbol{\phi}^g_\theta[s^g] \pi^g_{s^g}[\boldsymbol{p}] }{\sum_{\hat{\theta}\in\Theta}\boldsymbol{\mu}[\hat{\theta}] \sum_{\boldsymbol{p} \in \mathcal{P} : \boldsymbol{p}[i] = p_i'} \sum_{s^g \in \mathcal{S}^g : s^g_i = s_i'} \boldsymbol{\phi}^g_{\hat{\theta}}[s^g] \pi^g_{s^g}[\boldsymbol{p}] }.
\] 
\item $\boldsymbol{\xi}^h_{i, (s_i,p_i)} \in \Delta^{|\Theta|}$ posterior belief of a buyer $i \in \mathcal{N}$ upon receiving signal $s_i \in \mathcal{S}_i$ and price $\boldsymbol{p}[i]=p_i \in [0,1]$ when the price function is $h$, formally
\[
\boldsymbol{\xi}^h_{i, (s_i,p_i)}[\theta]=\frac{\boldsymbol{\mu}[\theta] \boldsymbol{\phi}^h_{i,\theta}[s_i] \pi^{h}_{s_i}[p_i] }{\sum_{\hat{\theta}\in\Theta}\boldsymbol{\mu}[\hat{\theta}] \boldsymbol{\phi}^h_{i,\hat{\theta}}[s_i] \pi^{h}_{s_i}[p_i] } = 
\frac{\boldsymbol{\mu}[\theta] \boldsymbol{\phi}^h_{i,\theta}[s_i]  }{\sum_{\hat{\theta}\in\Theta}\boldsymbol{\mu}[\hat{\theta}] \boldsymbol{\phi}^h_{i,\hat{\theta}}[s_i] } =
\boldsymbol{\xi}^h_{i, s_i}[\theta].\] 
\item $\boldsymbol{\xi}_{i, s_i} \in \Delta^{|\Theta|}$ posterior belief of a buyer $i \in \mathcal{N}$ upon receiving signal $s_i \in \mathcal{S}_i$ when the price function is $f$, formally
\[
\boldsymbol{\xi}_{i, s_i}[\theta]=\frac{\boldsymbol{\mu}[\theta] \boldsymbol{\phi}_{i, \theta}[s_i] }{\sum_{\theta'\in\Theta}\boldsymbol{\mu}[\theta'] \boldsymbol{\phi}_{i, \theta'}[s_i] }.
\]
\end{itemize}

For each couple $(s^g,\boldsymbol{p}) \in \mathcal{S}^g \times \mathcal{P}$ s.t. $\boldsymbol{p}[i]=p_i$ there exist a couple $(s^h_i,p_i) \in \mathcal{S}_i^h \times [0,1]$, the signaling scheme $\phi^h : \Theta \to \Delta^{|\mathcal{S}^h|}$ and the price function $h$ are such that \todog{check}
\[\boldsymbol{\xi}^h_{i, s^h_i}[\theta] = \boldsymbol{\xi}^g_{i, (s^{g},\boldsymbol{p})}[\theta],\]
that is:
\[\frac{\boldsymbol{\mu}[\theta] \boldsymbol{\phi}^h_{i,\theta}[s^h_i]  }{\sum_{\hat{\theta}\in\Theta}\boldsymbol{\mu}[\hat{\theta}] \boldsymbol{\phi}^h_{i,\hat{\theta}}[s^h_i] }= 
\frac{\boldsymbol{\mu}[\theta] \sum_{\boldsymbol{p} \in \mathcal{P} : \boldsymbol{p}[i] = p_i} \sum_{s^g \in \mathcal{S}^g} \boldsymbol{\phi}^g_\theta[s^g] \pi^g_{s^g}[\boldsymbol{p}] }{\sum_{\hat{\theta}\in\Theta}\boldsymbol{\mu}[\hat{\theta}] \sum_{\boldsymbol{p} \in \mathcal{P} : \boldsymbol{p}[i] = p_i} \sum_{s^g \in \mathcal{S}^g} \boldsymbol{\phi}^g_{\hat{\theta}}[s^g] \pi^g_{s^g}[\boldsymbol{p}] }.\]

This implies that the signaling scheme $\phi^h$ is s.t.
\[ \boldsymbol{\phi}^h_{i,\theta}[s^h_i] = \sum_{\boldsymbol{p} \in \mathcal{P} : \boldsymbol{p}[i] = p_i} \sum_{s^g \in \mathcal{S}^g} \boldsymbol{\phi}^g_\theta[s^g] \pi^g_{s^g}[\boldsymbol{p}].\]

We impose that signaling schemes $\phi^g: \Theta \rightarrow \Delta^{|\mathcal{S}^g|}$ and $\phi^h: \Theta \rightarrow \Delta^{|\mathcal{S}^h|}$ induces the same probability distribution over the posterior belief of buyer $i \in \mathcal{N}$
\[\boldsymbol{\gamma}[\boldsymbol{\xi}_i] =
\sum_{(s^g,\boldsymbol{p}) \in \mathcal{S}^g \times \mathcal{P}: \boldsymbol{\xi}_{i} = \boldsymbol{\xi}_{i,(s^g,\boldsymbol{p})} } \sum_{\theta \in \Theta} \boldsymbol{\mu}[\theta] \boldsymbol{\phi}^g_\theta[s^g] \pi^g_{s^g}[\boldsymbol{p}]=
\sum_{s^h_i \in \mathcal{S}^h_i: \boldsymbol{\xi}_{i} = \boldsymbol{\xi}_{i,s^h_i} } \sum_{\theta \in \Theta} \boldsymbol{\mu}[\theta] \boldsymbol{\phi}^h_{i, \theta}[s^h_i]
\hspace{1cm} \forall \boldsymbol{\xi}_i \in \Xi_i.\]

Notice that $|\mathcal{S}^h|=|\mathcal{S}^g| \times |\mathcal{P}|$.
The price function $h$ is such that 
\[\sum_{s^h_i \in \mathcal{S}^h_i} \pi^{h_i}_{s^h_i}[p_i] = \sum_{s^g \in \mathcal{S}^g} \sum_{\boldsymbol{p} \in \mathcal{P} : \boldsymbol{p}[i] = p_i} \pi^g_{s}[\boldsymbol{p}]\]

For each couple $(s^h_i,p_i) \in \mathcal{S}_i^h \times [0,1]$ there exist a couple $(s_i,p_i) \in \mathcal{S}_i \times [0,1]$, where $s_i \in \mathcal{S}_i$, the signaling scheme $\phi : \Theta \to \Delta^{|\mathcal{S}|}$ and the price function $f$ are such that $|\mathcal{S}_i|=|\mathcal{S}_i^h|\times |[0,1]|$, and
\[f(s_i)=p_i\]
and
\[\boldsymbol{\phi}_{i, \theta}[s_i] = \sum_{s^h_i \in \mathcal{S}^h_i}\boldsymbol{\phi}^h_{i, \theta}[s^h_i]\pi^{h}_{s^h_i}[p_i]\]

The signaling schemes $\phi^h: \Theta \rightarrow \Delta^{\mathcal{S}^h}$ and $\phi: \Theta \rightarrow \Delta^{\mathcal{S}}$ induces the same probability distribution over the posterior belief of buyer $i \in \mathcal{N}$

\[\boldsymbol{\gamma}[\boldsymbol{\xi}_i] =
\sum_{s^h_i \in \mathcal{S}^h_i: \boldsymbol{\xi}_{i} = \boldsymbol{\xi}_{i,s^h_i} } \sum_{\theta \in \Theta} \boldsymbol{\mu}[\theta] \boldsymbol{\phi}^h_{i, \theta}[s^h_i]=
\sum_{s_i \in \mathcal{S}_i: \boldsymbol{\xi}_{i} = \boldsymbol{\xi}_{i,s_i} } \sum_{\theta \in \Theta} \boldsymbol{\mu}[\theta] \boldsymbol{\phi}_{i, \theta}[s_i]
\hspace{1cm} \forall \boldsymbol{\xi}_i \in \Xi_i.\]

\subsection{Payment Function}

In the main paper, we consider a deterministic and factorized payment function $f:\mathcal{S}\rightarrow \mathcal{P}$ such that $f(\boldsymbol{s})=(f^i(s_i))_{i \in \mathcal{N}}$. 
Now, we prove in two steps that given a generic pair composed of a payment function and a signaling scheme, it is always possible to find another pair composed of a deterministic and factorized payment function, \emph{i.e.} $f$, and a signaling scheme inducing the same posted price auction. 
This means that the two scenarios provide the same revenue to the seller and the same posterior believes to the buyers. 
First, we show that for a generic stochastic payment function $g:\mathcal{S}^g\rightarrow \mathcal{P}$, where $\mathcal{S}^g \coloneqq \bigtimes_{i \in \mathcal{N}} \mathcal{S}^g_i$ is a set of signal profiles, we can find a factorized stochastic payment function $h:\mathcal{S}^h\rightarrow \mathcal{P}$, where  $\mathcal{S}^h \coloneqq \bigtimes_{i \in \mathcal{N}} \mathcal{S}^h_i$ is a set of signal profiles, inducing the same posted price auction. 
Then, we show that it is always possible to find a factorized deterministic payment function $f:\mathcal{S}\rightarrow \mathcal{P}$, where $\mathcal{S}\coloneqq \bigtimes_{i \in \mathcal{N}} \mathcal{S}_i$ is a set of signal profiles, inducing the same posted price auction of functions $g$ and $h$.

\paragraph{Notation}
\begin{itemize}
	\item $\mathcal{P}_i$ prices reserved for buyer $i$
	\item $\mathcal{P}\coloneqq \bigtimes_{i \in \mathcal{N}} \mathcal{P}_i$ set of price profiles $\boldsymbol{p}_j=(p_{j,1},\ldots,p_{j,n})$, where $j=\{1,\ldots,|\mathcal{P}|\}$
   \item $g:\mathcal{S}^g\rightarrow \mathcal{P}$ stochastic payment function
   \item $\mathcal{S}^g_i$ signals reserved for buyer $i$ when the payment function is $g$
   \item $\mathcal{S}^g$  set of signal profiles $\boldsymbol{s}^g_j=(s^g_{j,1},\ldots,s^g_{j,n})$, where $j=\{1,\ldots,|\mathcal{S}^g|\}$
   \item $\pi^g:\mathcal{S}^g\rightarrow \Delta^{|\mathcal{P}|}$ probability distribution induced by function $g$ over the prices profiles
   \item $\pi^g_{\boldsymbol{s}^g_j }[\boldsymbol{p}_k]$ probability of price profile $\boldsymbol{p}_k$ when the signal profile is $\boldsymbol{s}^g_j \in \mathcal{S}^g$ 
    \item $\pi^g_{\boldsymbol{s}^g_j }[p_{k,i}]$ probability of price $p_{k,i}$ for buyer $i$ when the signal profile is $\boldsymbol{s}^g_j \in \mathcal{S}^g$ 
    \[\pi^g_{\boldsymbol{s}^g_j }[p_{k,i}] = \sum_{\boldsymbol{p}_{\ell} \in \mathcal{P} : p_{\ell,i}=p_{k,i}} \pi^g_{\boldsymbol{s}^g_j }[\boldsymbol{p}_{\ell}]\]
   \item $h:\mathcal{S}^h\rightarrow \mathcal{P}$ stochastic factorized payment function, $h(\boldsymbol{s}^h_j)=(h^i(s^h_{j,i}))_{i \in \mathcal{N}}$
    \item $\mathcal{S}^h_i$ signals reserved for buyer $i$ when the payment function is $h$
   \item $\mathcal{S}^h$  set of signal profiles $\boldsymbol{s}^h_j=(s^h_{j,1},\ldots,s^h_{j,n})$, where $j=\{1,\ldots,|\mathcal{S}^h|\}$
   \item $\pi^h:\mathcal{S}^h\rightarrow \Delta^{|\mathcal{P}|}$ probability distribution induced by function $h$ over the prices profiles
   \item $\pi^h_{\boldsymbol{s}^h_j }[\boldsymbol{p}_k]$ probability of price profile $\boldsymbol{p}_k$ when the signal profile is $\boldsymbol{s}^h_j \in \mathcal{S}^h$ 
   \[ \pi^h_{\boldsymbol{s}^h_j }[\boldsymbol{p}_k] = \prod_{i\in \mathcal{N}} \pi^h_{s^h_{j,i}}[p_{k,i}]\]
   \item $\pi^g_{\boldsymbol{s}^h_j }[p_{k,i}]=\pi^h_{s^h_{j,i}}[p_{k,i}]$ probability of price $p_{k,i}$ for buyer $i$ when the signal profile is $\boldsymbol{s}^h_j \in \mathcal{S}^h$
    \item $f:\mathcal{S}\rightarrow \mathcal{P}$ deterministic factorized payment function, $f(\boldsymbol{s}_j)=(f^i(s_{j,i}))_{i \in \mathcal{N}}$
    \item $\mathcal{S}_i$ signals reserved for buyer $i$ when the payment function is $f$
    \item $\mathcal{S}$  set of signal profiles $\boldsymbol{s}_j=(s_{j,1},\ldots,s_{j,n})$, where $j=\{1,\ldots,|\mathcal{S}|\}$
    \item $\boldsymbol{\xi}^g_{i, (s^g_{j,i},p_{k,i})} \in \Delta^{|\Theta|}$ posterior belief of a buyer $i \in \mathcal{N}$ upon receiving signal $s^g_{j,i} \in \mathcal{S}^g_i$ and price $p_{k,i} \in \mathcal{P}$ when the price function is $g$, formally
    \[
    \boldsymbol{\xi}^g_{i, (s^g_{j,i},p_{k,i})}[\theta]=\frac{\boldsymbol{\mu}[\theta] \sum_{\boldsymbol{p}_{\ell} \in \mathcal{P} : p_{\ell,i} = p_{k,i}} \sum_{\boldsymbol{s}^g_m \in \mathcal{S}^g : s^g_{m,i} = s^g_{j,i}} \boldsymbol{\phi}^g_{\theta}[\boldsymbol{s}^g_m] \pi^g_{\boldsymbol{s}^g_m}[p_{k,i}]} {\sum_{\theta'\in\Theta}\boldsymbol{\mu}[\theta'] \sum_{\boldsymbol{p}_{\ell} \in \mathcal{P} : p_{\ell,i} = p_{k,i}} \sum_{\boldsymbol{s}^g_m \in \mathcal{S}^g : s^g_{m,i} = s^g_{j,i}} \boldsymbol{\phi}^g_{\theta'}[\boldsymbol{s}^g_m] \pi^g_{\boldsymbol{s}^g_m}[p_{k,i}] }.
    \] 
\end{itemize}

We denote by $\omega_i:\mathcal{S}^g \times \mathcal{P}_i \rightarrow \mathcal{S}^h_i $ a map from the cartesian product of sets $\mathcal{S}^g$ and $\mathcal{P}_i$ to the set $\mathcal{S}^h_i$. In particular, $\omega_i$ is defined as it Table~\ref{t:omega}.

\begin{table}[t!]
	\caption{Map $\omega_i:\mathcal{S}^g \times \mathcal{P}_i \rightarrow \mathcal{S}^h_i $.}
	\label{t:omega}
	\begin{center}
		%	{\renewcommand{\arraystretch}{1.0}
		\begin{tabular}{|c|c|}
			$(\boldsymbol{s}^g_j,p_{k,i})$ & $\omega(\boldsymbol{s}^g_j,p_{k,i})$ \\
			\hline
			\hline
			$(\boldsymbol{s}^g_1,p_{1,i})$ & $s^h_{1,i}$ \\
			\hline
			$(\boldsymbol{s}^g_1,p_{2,i})$ & $s^h_{2,i}$ \\
			\hline
			$\ldots$ & $\ldots$ \\
			\hline
			$(\boldsymbol{s}^g_1,p_{|\mathcal{P}_i|,i})$ & $s^h_{|\mathcal{P}_i|,i}$ \\
			\hline
			$(\boldsymbol{s}^g_2,p_{1,i})$ & $s^h_{|\mathcal{P}_i|+1,i}$ \\
			\hline
			$\ldots$ & $\ldots$ \\
			\hline
			$(\boldsymbol{s}^g_{|\mathcal{S}^g|},p_{|\mathcal{P}_i|,i})$ & $s^h_{|\mathcal{S}^g||\mathcal{P}_i|,i}$ \\
			\hline
		\end{tabular}	
	\end{center}
\end{table}

Notice that $|\mathcal{S}^h_i|=|\mathcal{S}^g||\mathcal{P}_i|$. 
The intuition is that, when the payment function is $g$, there may exist a relation between the price offered to buyer $i$ and the signals sent to any other buyer $j$, where $j \in \mathcal{N}$.
When the signaling scheme selects the signal profile $\boldsymbol{s}^g_j$ and the payment function select price profile $\boldsymbol{p}_{k}$, buyer $i$ observes signal $s^g_{j,i}$ and the price $p_{k,i}$. 
Signal $s^g_{j,i}$ is independent from other buyers' signals $s^g_{j,l}$, where $l \in \mathcal{N}\setminus\{i\}$. However, price $p_{k,i}$ depends on vector $\boldsymbol{s}^g_j$ (\emph{i.e.}, $g(\boldsymbol{s}^g_j)=p_{k,i}$), therefore, buyer $i$ may get some additional information w.r.t. that conveyed by signal $s^g_{j,i}$. 
In this scenario, the price is both a signal and the payment required by the posted price auction.
Conversely, when the payment function is $h$ and buyer $i$ observes signal $s^h_{j,i}$ and the price $p_{k,i}$, no additional information is conveyed by the price.  

First, we show that the two scenarios with payment functions $g$ and $h$ induce the same posterior believes.

\[\boldsymbol{\xi}^h_{i, s^h_i}[\theta] = \boldsymbol{\xi}^g_{i, (s^{g},\boldsymbol{p})}[\theta],\]

\begin{align}
\boldsymbol{\xi}^g_{i, (\boldsymbol{s}^g_j,p_{k,i})}[\theta] = 
\end{align}
